# Supplementary material for: Event-Triggered Diffusion Kalman Filters
Source: arXiv:1711.00493 source file (2020-02-18)
Supplement: Supplementary file 1 [file appendix_tsang.tex]

\section*{Appendix}

  \begin{table}[htb]
\begin{center}
\begin{tabular}{ c|| c| c| c }
 & Step 1 & Step 2 & Step 3  \\ 
 \hline \hline

$P$ & Increase  & Decrease & No Change \\
$\Sigma$ & Increase & Decrease \cite{conf:kalconv,conf:avgconsensus4} & Governed by (\ref{eq:step3}) \\
\end{tabular}
\end{center}
\caption{Summary of the effect of each step of  Diffusion Kalman Filter on $P$ and $\Sigma$ }
\end{table}
%One of the Kalman filter assumption is that the underlying random variables (r.v.s) are Gaussian. However, in nonlinear case (where the EKF applies), even though the initial r.v.s are Gaussian, after one nonlinear time-update, it is no longer Gaussian, and it is meaningless to discuss its covariance. Therefore, when applying EKF, we all assume that the nonlinear effect is minor, and after whatever updates, the underlying r.v.s are still Gaussian.

%Another issue that have to consider in EKF is that the update rules depend on the state (measurement matrix etc.). However, we already get rid of this problem in the theoretical analysis part. In other words, in terms of EKF, we already address everything we know, and the left is not what we can deal with.
Inherent in the original centralized Kalman filter a powerful tool which error covariance matrix. It is well maintained and time updated by the underlying core of Kalman filter. Such a covariance is a perfect measure of the estimated accuracy of the state. However, when it comes to the distributed diffusion Kalman filter, it is important to note it lost such nice feature. Thus the covariance of the estimation error is not available locally anymore, since the diffusion update does not take into account the recursions for the covariance, and it messes up the notion of the state error.

Therefore, one of the main problems in diffusion Kalman filter is that the matrix $P_k$ used in every local nodes is not necessarily the real covariance. Even though one collects all $P_k$'s, one still can not reconstruct the overall covariance of the system $\Sigma=E[\tilde{\mathcal{X}}\tilde{\mathcal{X}}^T]$. While the triggering event is defined on local $P_k$, we need to address the relation between $P_k$ and $\Sigma$ for clarity. We discuss three steps of diffusion Kalman filter in the following.
%\begin{itemize}

\subsection{\textbf{Step 1}: Time update}
Every local $P_k$ updates by
$P_{k,t+1|t} = \bar{F}_i(\hat{x}^k_{t|t})P_{k,t|t}\bar{F}_i(\hat{x}^k_{t|t})^* + Q_t$. 
In terms of local Kalman filter, one has 
\begin{equation}
   tr(W P_{k,i+1|i} W^T) \geq tr(W P_{k,i|i} W^T)
   \label{eq:P_increase}
\end{equation}
with $W$ defined in (11) and $Q_i \geq 0$ in positive-semidefinite sense.
While the overall covariance is updated by $ \Sigma_{t+1|t} = \mathcal{F} \Sigma_{t|t} \mathcal{F}^* + Q$, we have 
\begin{equation}
\sum_{i=0}^{N-1}tr(W \Sigma_{k,i+1|i} W^T) \geq \sum_{i=0}^{N-1} tr(W \Sigma_{k,i|i} W^T).
   \label{eq:sigma_increase}
\end{equation}

\subsection{\textbf{Step 2}: Measurement update}
$P_k$ updates according to 
\[
   P^{-1}_{k,t|t}= P^{-1}_{k,t|t-1} + \sum\limits_{j\in\mathcal{N}_{k}}\hat{H}_{kj,t}^* {R}^{-1}_t \hat{H}_{kj,t},
\]
as in standard Kalman filter and one arrives $P_{k,t|t} \leq P_{k,t|t-1}$.
However, the overall covariance $\Sigma$ updates by
   \begin{equation}
   \Sigma_{t|t} =  \mathcal{P}_{t|t} \mathcal{P}_{t|t-1}^{-1} \Sigma_{t|t-1} \mathcal{P}_{t|t-1}^{-1}  \mathcal{P}_{t|t} + \mathcal{P}_{t|t} \mathcal{L}^{\T}\mathcal{H}^* R^{-1}\mathcal{H}  \mathcal{L}\mathcal{P}_{t|t}.
   \label{eq:step2}
   \end{equation}
The covariance should decrease as in \cite{conf:kalconv,conf:avgconsensus4}. However, we do not prove this in this work.

\subsection{\textbf{Step 3}: Diffusion update}
In diffusion Kalman filter, local $P_k$'s are not varied in this step, even though the estimations are changed. Correspondingly, the overall covariance changes by
  \begin{equation}
      \Sigma_{t^+} =  \mathcal{C}^{\T}\Sigma_{t^-} \mathcal{C}.
      \label{eq:step3}
   \end{equation}
   However, the order of $\Sigma_{t^+}$ and $\Sigma_{t^-}$ can not be guaranteed in general.

The tentative result can be summarized in Table I. While diffusion update is widely applied, the interplay between local and global estimations needs to be explored furthermore.

 % $P$ & Increase by (\ref{eq:P_increase}) & decrease & invariant \\
%  $\Sigma$ & increase by (\ref{eq:sigma_increase}) & characterized by (\ref{eq:step2})  & characterized by (\ref{eq:step3}) \\
