# Supplementary material for: Event-Triggered Diffusion Kalman Filters
Source: arXiv:1711.00493 source file (2020-02-18)
Supplement: Supplementary file 2 [file appendix.tex]

%\begin{figure}[tb]
%\centering
%\includegraphics[width = 0.5\textwidth]{Figures/testbed_v2.jpg}
%\caption{(a) CrazyFlie 2.0 helicopter equipped with the very same Decawave ultra-wideband radio, (b) Ceiling-mounted anchor node
%, and (c) Custom ranging anchor circuit board}
%\label{fig:testbed}
%\end{figure}

%\section{Experimental Setup}
\section*{Appendix}
%We evaluated the performance of the proposed event-triggered algorithm on a custom ultra-wideband RF test bed based on the DecaWave DW1000 IR-UWB radio \cite{dw1000}. The overall setup is shown in Figure \ref{fig:full_sys}. The main components of our test-bed can be summarized in the following points.
% 
